# Supplementary material for: A robust model-based clustering based on the geometric median and the Median Covariation Matrix
Source: arXiv:2211.08131 source file (2022-11-15)
Supplement: Supplementary file 2 [file appendixTabGMM1500C0.tex]

\begin{figure}[ht]
  \begin{center}
    \begin{tabular}{c|cc}
      {scenario ($a$): outliers $U$} &
      {scenario ($b$): outliers $T_1(0)$} & 
      {scenario ($c$): outliers $T_1(\mu_k)$} \\
      \includegraphics[width=.22\textwidth, trim=10 10 10 50, clip=]{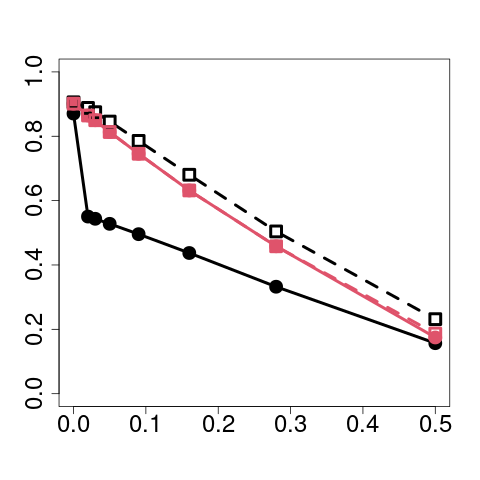} &
      \includegraphics[width=.22\textwidth, trim=10 10 10 50, clip=]{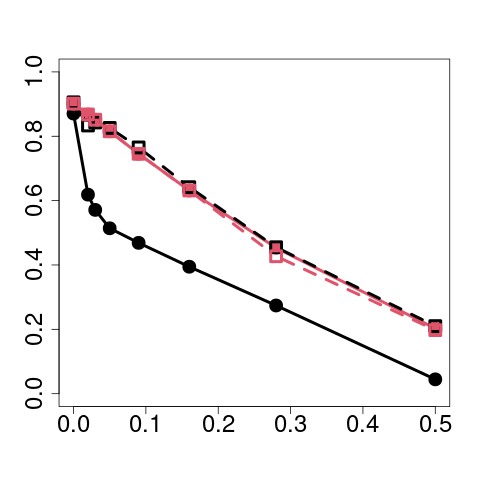} &
      \includegraphics[width=.22\textwidth, trim=10 10 10 50, clip=]{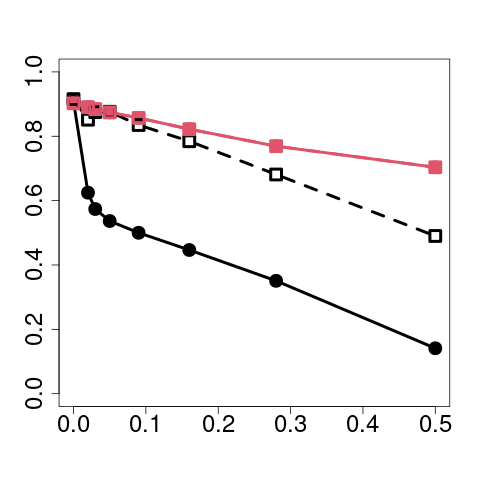} \\
      \hline
      & & \\
      & 
      {scenario ($d$): outliers $T_2(0)$} &
      {scenario ($e$): outliers $T_2(\mu_k)$} \\
      &
      \includegraphics[width=.22\textwidth, trim=10 10 10 50, clip=]{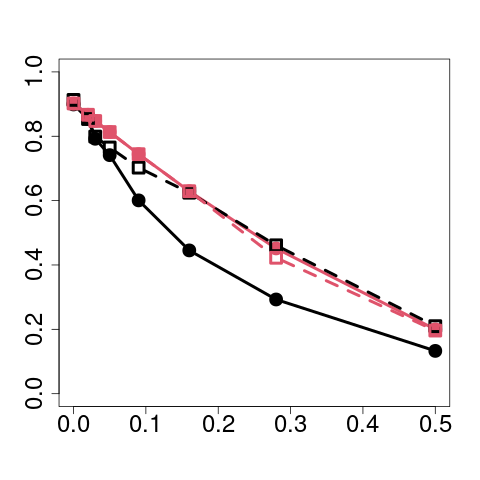} &
      \includegraphics[width=.22\textwidth, trim=10 10 10 50, clip=]{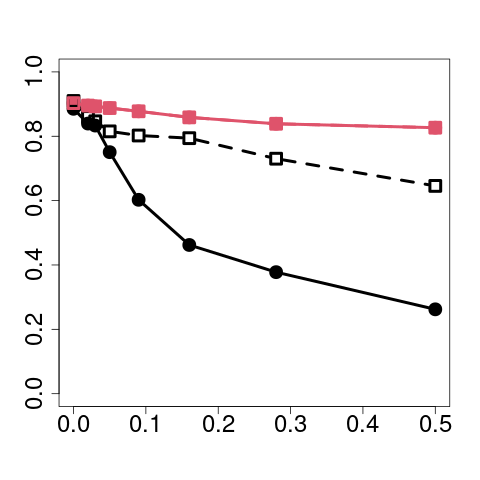} 
    \end{tabular}
    \caption{Gaussian mixture model: classification accuracy ($ARI$), when considering only non-outlier observations. Same legend as Figure \ref{fig:simGMMclassif1500}. \label{fig:simGMMsupp}}
  \end{center}
\end{figure}
