# Supplementary material for: A robust model-based clustering based on the geometric median and the Median Covariation Matrix
Source: arXiv:2211.08131 source file (2022-11-15)
Supplement: Supplementary file 4 [file appendixTabTMM150.tex]

\begin{figure}[ht]
  \centering
%   \begin{center}
    \begin{tabular}{c|m{.2\textwidth}m{.2\textwidth}|m{.2\textwidth}m{.2\textwidth}}
      & 
      \multicolumn{2}{c|}{Classification} & 
      \multicolumn{2}{c}{Parameter estimation} \\ 
      &
      \multicolumn{1}{c}{ARI} & \multicolumn{1}{c|}{$\widehat{K}$} & 
      \multicolumn{1}{c}{$MSE(\mu)$} & \multicolumn{1}{c}{$MSE(\Sigma)$} \\ 
      \hline
%       & & & \\
      ($a$) &
      \includegraphics[width=.2\textwidth, trim=10 10 10 50, clip=]{figures/simRTMM-p5-K3-n150-s1-ARI} &
      \includegraphics[width=.2\textwidth, trim=10 10 10 50, clip=]{figures/simRTMM-p5-K3-n150-s1-K} &
      \includegraphics[width=.2\textwidth, trim=10 10 10 50, clip=]{figures/simRTMM-p5-K3-n150-s1-MSEmu} &
      \includegraphics[width=.2\textwidth, trim=10 10 10 50, clip=]{figures/simRTMM-p5-K3-n150-s1-MSEsigma} \\
      ($b$) &
      \includegraphics[width=.2\textwidth, trim=10 10 10 50, clip=]{figures/simRTMM-p5-K3-n150-s2-ARI} &
      \includegraphics[width=.2\textwidth, trim=10 10 10 50, clip=]{figures/simRTMM-p5-K3-n150-s2-K} &
      \includegraphics[width=.2\textwidth, trim=10 10 10 50, clip=]{figures/simRTMM-p5-K3-n150-s2-MSEmu} &
      \includegraphics[width=.2\textwidth, trim=10 10 10 50, clip=]{figures/simRTMM-p5-K3-n150-s2-MSEsigma} \\
      ($c$) &
      \includegraphics[width=.2\textwidth, trim=10 10 10 50, clip=]{figures/simRTMM-p5-K3-n150-s3-ARI} &
      \includegraphics[width=.2\textwidth, trim=10 10 10 50, clip=]{figures/simRTMM-p5-K3-n150-s3-K} &
      \includegraphics[width=.2\textwidth, trim=10 10 10 50, clip=]{figures/simRTMM-p5-K3-n150-s3-MSEmu} &
      \includegraphics[width=.2\textwidth, trim=10 10 10 50, clip=]{figures/simRTMM-p5-K3-n150-s3-MSEsigma} \\
      ($d$) &
      \includegraphics[width=.2\textwidth, trim=10 10 10 50, clip=]{figures/simRTMM-p5-K3-n150-s4-ARI} &
      \includegraphics[width=.2\textwidth, trim=10 10 10 50, clip=]{figures/simRTMM-p5-K3-n150-s4-K} &
      \includegraphics[width=.2\textwidth, trim=10 10 10 50, clip=]{figures/simRTMM-p5-K3-n150-s4-MSEmu} &
      \includegraphics[width=.2\textwidth, trim=10 10 10 50, clip=]{figures/simRTMM-p5-K3-n150-s4-MSEsigma} \\
      ($e$) &
      \includegraphics[width=.2\textwidth, trim=10 10 10 50, clip=]{figures/simRTMM-p5-K3-n150-s5-ARI} &
      \includegraphics[width=.2\textwidth, trim=10 10 10 50, clip=]{figures/simRTMM-p5-K3-n150-s5-K} &
      \includegraphics[width=.2\textwidth, trim=10 10 10 50, clip=]{figures/simRTMM-p5-K3-n150-s5-MSEmu} &
      \includegraphics[width=.2\textwidth, trim=10 10 10 50, clip=]{figures/simRTMM-p5-K3-n150-s5-MSEsigma} 
    \end{tabular}
    \caption{Student mixture model: classification accuracy ($ARI$), estimated number of clusters $\widehat{K}$, estimation error fu the mean ($MSE(\mu)$) and for the variance ($MSE(\Sigma)$) for scenarios ($a$) to ($e$), with $n_k = 50$ observation in each of the $K^*$ clusters ($n = 150$). Same legend as Figure \ref{fig:simGMM1500}. \label{fig:simTMM150}}
%   \end{center}
\end{figure}
